# Supplementary material for: Maximum Mean Discrepancy Distributionally Robust Nonlinear Chance-Constrained Optimization with Finite-Sample Guarantee
Source: arXiv:2204.11564 source file (2022-04-25)
Supplement: Supplementary file 1 [file appendix.tex]

\section{Proofs}
\label{sec:proof}
In this section we provide the proof for Theorem \ref{thm:exact} where we introduced the exact reformulation of the feasible set $Z$ in \eqref{eq:set_z}.
\begin{proof}
Start by replacing $\inf_{\mathbb P \in \mathcal P} \mathbb P [f(x, \xi) \leq 0] \geq 1 - \alpha$ with the equivalent $\sup_{\mathbb P \in \mathcal P} \mathbb P [f(x, \xi) > 0] \leq \alpha$.
Next we can rewrite the probability with an indicator function
$$
\mathbb P [f(x, \xi) > 0] = \mathbb E_\mathbb{P} [\mathbb 1\big(f(x, \xi) > 0\big)].
$$
We note that the indicator function fulfills the assumptions on the constraint function of the strong duality result, therefore according to \cite[Theorem 3.1]{zhuKernelDistributionallyRobust2020} we rewrite
$$
\sup_{\mathbb P \in \mathcal P} \mathbb E_\mathbb{P} [\mathbb 1\big(f(x, \xi) > 0\big)]
$$ as
\begin{alignat}{2}
& \min_{g\in \mathcal H} \quad && \frac{1}{N}\sum_{i=0}^N g(\xi_i) + \epsilon ||g||_{\mathcal H}\\
& \text{subject to} \quad && \mathbb 1\big(f(x, \xi) > 0\big) \leq g(\xi) \quad \forall \xi \in \Xi.
\end{alignat}
Plugging these reformulations back into \eqref{eq:set_z}, the set $Z$ then becomes
\begin{empheq}[left=Z \coloneqq \left\{ x \in \mathbb R^n :, right=\right\} ]{align}
    &\frac{1}{N} \sum_{i=0}^N g(\xi_i) + \epsilon ||g||_{\mathcal H} \leq \alpha \\
    &\mathbb 1(f(x, \xi) > 0) \leq g(\xi) \, \forall \xi \in \Xi\\
    &g \in \mathcal H
\end{empheq}
    % \begin{equation}
    %     Z \coloneqq \big\{ x \in \mathbb R^n: \mathbb E_{\hat{\mathbb P}} g(\xi) + \epsilon ||g||_{\mathcal H} \leq \alpha, \mathbb 1(f(x, \xi_i) \leq 0) \leq g(\xi_i) \, \forall i = 1, \dots, M, \exists g \in \mathcal H \big\}
    % \end{equation}
\end{proof}

\subsection{Tractable reformulation}
\jz{Let's move this whole section to the appendix, just leave one statement. It should look like "Example 3.4" in my paper\url{https://arxiv.org/pdf/2006.06981.pdf} The reason is that the tractable reformulation might even hurt our contribution. There is not point doing MMD constraints when using this kernel you choose. So an example showing connection is enough. Moreover, the SVM connection, if established clearly, can also serve as such an "example" here.}
\label{ass:pw_affine}
Under the following assumptions, we will present a tractable reformulation of the $\CVaR$ relaxation.
\begin{assume}
Let the constraint function $f(x, \xi)$ be piesewise-affine in the uncertainty $\xi$ $f(x, \xi) = \max_{k \in [K]} x^T A_k \xi + b_k(x)$, for some positive integer $K$ and $A_k \in \mathbb R^{n\times m}$ and $b_k(x): \mathbb R^n \mapsto \mathbb R$ some convex function. Further we assume that the uncertainty is supported on a closed convex set $\Xi = \{\xi \in \mathbb R^m : C\xi \leq h\}$.
\end{assume}
The following derivation of Proposition takes inspiration from \cite{hotaDataDrivenChanceConstrained2018, MohajerinEsfahani2018, guDistributionallyRobustChanceConstrained2021}.
\begin{proposition}
Let the constraint function $f$ and the support $\Xi$ of the uncertainty fulfil the assumptions in \ref{ass:pw_affine}. Let the ambiguity set $\mathcal P$ be defined as in \eqref{eq:amb_set}. Then the feasible set in \eqref{eq:z_cvar} is equivalent to the following set

\begin{subequations}
    \label{eq:lin_cvar}
    \begin{empheq}[left={%
    \begin{aligned}[b]
         &\mathrlap{Z_{\CVaR}\coloneqq}\\ \\ \\ \\[2ex]
         & \quad
    \end{aligned}
    \empheqlbrace x \in \mathbb R^n:}, right=\empheqrbrace]
    {align}
    & g_0 + \frac{1}{N} \sum_{i=1}^N g(\xi_i) + \varepsilon ||g||_\rkhs \leq t \alpha \\
    & h^T y_1 + \beta^T \mathbf 1 + b_k(x) + t - g_0 \leq 0
    \label{subeq:k2}\\
    & C^Ty_1 = x^T A_k - \beta^T (\xi_1, \dots, \xi_N)^T 
    \label{subeq:k1}\\
    & h^T y_2 + \beta^T \mathbf 1 - g_0 \leq 0 \\
    & C^T y_2 = -\beta ^T (\xi_1, \dots, \xi_N)^T \\
    & t \geq 0,
    \end{empheq}
\end{subequations}
where \eqref{subeq:k2} and \eqref{subeq:k1} hold for all $k \in [K]$ and we parametrize $g(\xi)$ using a linear kernel as $g(\xi) = \sum_{i=}^N \beta_i (\langle \xi_i, \xi \rangle + 1$). This reformulation is convex in $x$ and linear in all other variables.
\end{proposition}
\begin{proof}
Note that
$$[f(x, \xi) + t]_+ \leq g_0 + g(\xi) \quad \forall \xi \in \Xi$$
is equivalent to
\begin{align}
\label{eq:lin_maj}
&\sup_{\xi \in \Xi} [f(x, \xi) - g(\xi)] + t - g_0 \leq 0 \\
\label{eq:lin_pos}
&\sup_{\xi \in \Xi} -g(\xi) -g0 \leq 0    
\end{align}
We can now plug in our hypotheses form Assumption \ref{ass:pw_affine} such that after some trivial reformulations we obtain the following
\begin{align*}
b_k(x) + t - g_0 + \sup_{C\xi \leq h} [x^TA_k \xi - g(\xi)] \leq 0\\
-g_0 + \sup_{C\xi \leq h} -g(\xi) \leq 0.
\end{align*}
In order to further simplify the inner supremum, we can use the fact that the constraint is affine in $\xi$ and therefore parametrize $g(\xi)$ using a linear kernel $k(\xi, \xi') = \langle \xi, \xi' \rangle + 1$ as $g(\xi) = \sum_{i=1}^N \beta_i k(\xi_i, \xi)$, following the robust representer formulation in \cite[Lemma B.1]{zhuKernelDistributionallyRobust2020}. Note that with that parametrization the problem now is linear in $\xi$. We can then write down the dual problems for the supremum in both cases such that be obtain
\begin{align*}
& \beta^T \mathbf 1 + b_k(x) + t - g_0 + \inf_{\substack{y_1 \geq 0 \\ C^T y_1 = x^TA_k - \beta^T(\xi_1, \dots, \xi_N)^T}} h^Ty_1 \leq 0\\
& \beta^T \mathbf{1} - g_0 + \inf_{\substack{y_2 \geq 0 \\ C^T y_2 = -\beta^T (\xi_1, \dots, \xi_n)^T}} h^T y_2 \leq 0
\end{align*}
When plugging these two dual problems back into the feasible set we can drop the $\inf$ in both cases, since both equations only hold if and only if $y_1, y_2 \geq 0$ exist such that infimum is achieved and equality constraints are fulfilled. \yassine{Ask JJ what happens is inf not achieved and equal to $-\infty$.}
\end{proof}

\section{Appendix}
%%%%%%%%%%%%%%%%%%%%%%%%%%%%%%%%%%%%%%%%%%%%%%%%%%%%%%%%%%%%%%%%%%%%%%%%%%%%%%%%%%%%%%%
% Mixed-Integer relaxation section
\subsection{Mixed Integer relaxation}
\label{subsec:MIP}
\yassine{While the reformulation holds for general constraints $f(x, \xi)$, solvers can only handle affine constraints. So, it seems a bit misleading to not mention this.} \heiner{The requirement is only on $x$ right? I think the dependence on $\xi$ can still be arbitrarily non-linear. Should probably make clearer everywhere when we refer to properties w.r.t.\ $x$ and when w.r.t.\ $\xi$.}
Off-the-shelf numerical solvers cannot handle the characteristic function in \eqref{eq:characteristic}. Therefore, we relax the set $Z$ in Theorem \ref{thm:exact} to a mixed integer representation. To this end, we introduce two binary variables $\mu_i^{(0)}, \mu_i^{(1)} \in \{0, 1\}$ for every $\xi_i$ in $\{\xi_i\}_{i=1}^N$, and a big-M coefficient $M$ \cite{REFS} \yassine{How about \cite{songChanceConstrainedBinaryPacking2014}, they use it a lot. But not a text book.}. We can then relax the inequality with the characteristic function in \eqref{eq:characteristic} to the inequalities in \cref{eq:MIvio,eq:MIacc,eq:sum,eq:majorant,eq:binary}.
\yassine{Add proof.}
\begin{proposition}
\label{prop:mip}
Suppose there exists a constant $M \in \mathbb R_+$ such that 
$$
\max_{x\in Z} |f(x, \xi_i)| \leq M, \quad i=1, \dots, N.
$$
Then the exact reformulation of the feasible set $Z$ in Theorem \ref{thm:exact} can be approximated by the mixed integer representation $Z_{\text{MIP}}$, with
\begin{subequations}
    \label{eq:MIrep}
    \begin{empheq}[left=Z_{\text{MIP}} \coloneqq \left\{ x \in \mathbb R^n :, right=\right\} ]{align}
        &\mathbb E_{\hat{\mathbb P}} g(\xi) + \epsilon ||g||_{\mathcal H} \leq \alpha \label{eq:exp_emp}\\
        &f(x, \xi_i) \geq -(1 - \mu_i ^{(1)})M, \label{eq:MIvio}\\
        &f(x, \xi_i) \leq (1 - \mu_i ^{(2)})M, \label{eq:MIacc}\\
        &\sum_{j=1}^2 \mu_i^{(j)} = 1, \label{eq:sum}\\
        &g(\xi_i) \geq \mu_i^{(1)}, \label{eq:majorant}\\
        &\mu_i^{(j)} \in \{0, 1\}, \label{eq:binary}
    \end{empheq}
\end{subequations}
where the indices $i = 1, \dots, N$ and  $j=1, 2$ if not further specified.
\end{proposition}
%We note that \eqref{eq:dual_exist} holds since we know that the infimum in \eqref{eq:zcvar} is attained. \yn{Ask JJ about this. In \cite{hotaDataDrivenChanceConstrained2018} they restate the strong duality theorem for wasserstein and that there exists a finite solution. I assume something similar should hold for our case.}

\heiner{Need some further discussion here. Under what conditions does the MIP solution converge to the true solution? How do we choose $M$?}
